# Supplementary material for: Perturbed Decision-Focused Learning for Modeling Strategic Energy Storage
Source: arXiv:2406.17085 source file (2024-12-05)
Supplement: Supplementary file 1 [file Appendix2.tex]

\newpage
 \section*{Supplementary Material}

%Our paper extensively employs Gamma and Beta distributions. Here

\subsection{Gamma and Beta distributions}
We briefly introduce Gamma and Beta distributions. The Gamma function 

\begin{equation}\Gamma(e_0)=\int_0^{\infty}x^{e_0-1}e^{-x} dx
\end{equation}
The Gamma distribution is defined as follows:
\begin{equation}
    \Gamma(\gamma_{\epsilon}|e_0,f_0)=\frac{{f_0}^{e_0}(\gamma_{\epsilon})^{e_0-1}e^{-f_0 \gamma_{\epsilon}}}{\Gamma(e_0)} \propto (\gamma_{\epsilon})^{e_0-1}e^{-f_0 \gamma_{\epsilon}}}
\end{equation}
  where  $e_0>0, f_0>0$, \propto$ means ``proportional to''.
   The notation $\Gamma(\gamma_{\epsilon}|e_0,f_0)$ means that $\gamma_\epsilon$ follows a Gamma distribution with parameters $e_0$ and $f_0$. The same rule applies to other notations in the following. 
The mean for this Gamma distribution is $e_0 /f_0$ and the variance is $e_0 /{f_0}^2$. \\

The Beta distribution is defined as: 
\begin{equation}
    \text{Beta}(\pi_k^c|\alpha, \beta)=\frac{\Gamma(\alpha+\beta)}{\Gamma(\alpha)\Gamma(\beta)}(\pi_k^c)^{\alpha-1}(1-\pi_k^c)^{\beta-1}
\end{equation}
The mean is $\frac{\alpha}{\alpha+\beta}$ and the variance is $\frac{\alpha \beta}{(\alpha+\beta)^2(\alpha+\beta+1)}$.

\subsection{Updating rule for Gibbs sampling}
The full probability of the parameters and the recorded data with all the labels  $P(\bm{\Theta}, \bm{X}, \bm{Y})$ based on the prior is characterized by (\ref{fullliklihood1}).
%The full likelihood of proposed model is expressed in 

\begin{equation} \label{fullliklihood1}
\begin{split}
%&P(\bm{X},\bm{Y},\bm{D},\bm{Z},\bm{S},\bm{\pi},\bm{\phi},\bm{\gamma_s},\gamma_{\epsilon})=\\
P(\bm{\Theta}, \bm{X}, \bm{Y})=&\prod_{i=1}^N \mathcal{N}(\bm{x}_i|\sum_{c=1}^{C}\bm{D}^c (\bm{z}_i^c \odot \bm{s}_i^c) y_i^c,\frac{1}{\gamma_{\epsilon}} \bm{I}_P)  \\
&\prod_{c=1}^C \prod_{i=1}^N \mathcal{N}(\bm{s}_i^c|0,\frac{1}{\gamma_s^c} \bm{I}_{K_c})\text{Bernoulli}(y_i^c|\phi^c) \\
&\prod_{c=1}^C\prod_{k=1}^{K_c} \mathcal{N}(\bm{d}_k^c|0,\lambda_d^{-1} \bm{I}_P) \text{Beta}(\pi_k^c|a_0,b_0)\\
&\prod_{c=1}^C \prod_{i=1}^N\prod_{k=1}^{K_c}\text{Bernoulli}(z_{ik}^c|\pi_k^c) \\
&\prod_{c=1}^C \Gamma(\gamma_s^c|c_0,d_0) \text{Beta}(\phi^c|g_0,h_0)\Gamma(\gamma_\epsilon|e_0,f_0) 
\end{split}
\end{equation}
 $\mathcal{N}(\bm{x}_i|\sum_{c=1}^{C}\bm{D}^c (\bm{z}_i^c \odot \bm{s}_i^c) y_i^c,\frac{1}{\gamma_{\epsilon}} \bm{I}_P)$ 
means that when   $\bm{D}^c$, $\bm{z}_i^c$,  $\bm{s}_i^c$, $y_i^c$ are all given,  $\bm{x}_i$ follows a Gaussian distribution with mean $\sum_{c=1}^{C}\bm{D}^c (\bm{z}_i^c \odot \bm{s}_i^c) y_i^c$ and covariance $\frac{1}{\gamma_{\epsilon}} \bm{I}_P$.

 \iffalse
 is the likelihood of $\bm{x}_i$. The likelihood is how we believe our data is generated. Because $\bm{x}_i = \sum_{c=1}^{C}\bm{D}^{c} \bm{\omega}_i^c+\bm{\epsilon}_i $ and $\bm{\epsilon}_i \sim \mathcal{N}(\bold{0},\frac{1}{\gamma_{\epsilon}} \bm{I}_P)$. Thus, we assume $\bm{x}_i$ is generated from a Gaussian distribution with mean  $\sum_{c=1}^{C}\bm{D}^c (\bm{z}_i^c \odot \bm{s}_i^c) y_i^c$ and variance $\frac{1}{\gamma_{\epsilon}} \bm{I}_P$.  Other distributions in  hierarchical model (\ref{fullliklihood1}) are the prior distributions we placed in (1)-(11).  
\fi

Then the updating rules in Gibbs Sample are shown below.

\noindent (I) The posterior distribution over $\bm{d}_{p.}$ (for all $p=1,..., mn_2$), the $p$th row of dictionary, is a Gaussian distribution with mean $E[{\bm{d}_{p.}}]$ and covariance $\bm{\Sigma}_{\bm{d}_{p.}}$, i.e., 
\begin{equation} \label{updateD}
q(\bm{d}_{p.}) \sim  \mathcal{N}(E[\bm{d}_{p.}],\bm{\Sigma}_{\bm{d}_{p.}})
\end{equation}

where

 \begin{equation} \label{updateD1}
&\bm{\Sigma}_{\bm{d}_{p.}}={[{E[\gamma_\epsilon]}\sum_{q: (p,q) \in \Psi_{\Omega} }  E[(\bm{s}_{.q} \odot \bm{z}_{.q}) (\bm{s}_{.q}\odot \bm{z}_{.q})^{T}] \\
&+\lambda_{d} I_{K}]^{-1} 
\end{equation}

\begin{equation} \label{updateD2}
\begin{split}
E[\bm{d}_{p.}]={E[\gamma_\epsilon}] \sum_{q: (p,q) \in \Psi_{\Omega}} \mathcal{H}$(Y-E)_{p,q}(E[\bm{s}_{.q}]^T\odot E[\bm{z}_{.q}]^T) \bm{\Sigma}_{\bm{d}_{p.}}
  \end{split}
\end{equation}
 $\Psi_{\Omega}$ denotes the set of observed entries in observed hankel matrix $Y^{o}$ 
 
And 
\begin{equation}
\begin{split}
&E[(\bm{s}_{.q} \odot \bm{z}_{.q}) (\bm{s}_{.q}\odot \bm{z}_{.q})^{T}]=E[\bm{s}_{.q}\bm{s}_{.q}^T] \odot E[\bm{z}_{.q}\bm{z}_{.q}^T]\\
&=(E[\bm{s}_{.q}]E[\bm{s}_{.q}]^T+\bm{\Sigma}_{\bm{s}_{.q}} )\odot (E[\bm{z}_{.q}]E[\bm{z}_{.q}]^T+\bm{\Sigma}_{\bm{z}_{.q}} )
  \end{split}
\end{equation}

$\bm{\Sigma}_{z_{.q}}=\text{diag}[E[z_{1q}](1-E[z_{1q}]),...,E[z_{Kq}](1-E[z_{Kq}])]$

\noindent(II) The posterior distribution $\bm{s}_{.q}$ ($q=1,...,n_1$ and $k=1,..., K$) 
is a Gaussian distribution 

\begin{equation} \label{updateS}
q({\bm{s}_{.q}}) \sim  \mathcal{N}(E[{\bm{s}_{.q}}],\bm{\Sigma}_{\bm{s}_{.q}})
\end{equation}
where
\begin{equation}\label{updateS1}
\bm{\Sigma}_{\bm{s}_{.q}}=[E[\gamma_{\epsilon}] \sum_{p:(p,q)\in \Psi_\Omega}E[\bm{\phi}_{p,q}^T\bm{\phi}_{p,q}]+E[\gamma_s] I_K]^{-1} 
\end{equation}

\begin{equation}\label{updateS2}
E[\bm{s}_{.q}]={E[\gamma_{\epsilon}]} \bm{\Sigma}_{\bm{s}_{.q}} \sum_{p:(p,q) \in \Psi_{\Omega}} E[\bm{\phi}_{p,q}]^{T}  \mathcal{H}(\bm{Y}-\bm{E})_{p,q}
\end{equation}

And $E[\bm{\phi}_{p,q}]= E[\bm{d}_{p.}] \odot E[\bm{z}_{.q}]^{T}$

\begin{equation}
\begin{split}
&E[\bm{\phi}^T \bm{\phi}] = (E[\bm{d}_{p.}^T\bm{d}_{p.}])\odot (E[\bm{z}_{.q}^T\bm{z}_{.q}]) \\
&= (E[\bm{d}_{p.}]^TE[\bm{d}_{p.}]+\Sigma_{\bm{d}_{p.}})\odot (E[\bm{z}_{.q}]E[\bm{z}_{.q}]^T+ \bm{\Sigma}_{\bm{z}_{.q}}))
  \end{split}
\end{equation}

\noindent(III)The approximation distribution over $z_{kq}$ (for all $q=1,...,n_1$, and $k=1,..., K$) is a Bernoulli distribution
\begin{equation} \label{updateZ}
q(z_{kq})\sim \text{Bernoulli}(\frac{\text{{q}}(z_{kq}=1)}{ \text{{q}}(z_{kq}=1)+\text{{q}}(z_{kq}=0)})
\end{equation}

with mean and variance,

\begin{equation}\label{updateZ1}
E[z_{kq}]=\frac{\text{{q}}(z_{kq}=1)}{ \text{{q}}(z_{kq}=1)+\text{{q}}(z_{kq}=0)}
\end{equation}

\begin{equation}\label{updateZ2}
\bm{\Sigma}_{z_{kq}}=E[z_{kq}](1-E[z_{kq}])
\end{equation}

where

\begin{equation}
\begin{split}
&\text{ln}(\text{\bf{q}}(z_{kq}=1)) \propto\\ &\frac{-E[\gamma_\epsilon]}{2} \sum_{p:(p,q)\in \Psi_{\Omega}}[\text{trace}(E[\bm{d}_{p.}^T\bm{d}_{p.}](E[\bm{s}_{.q} \bm{s}_{.q}^T ] \odot E[\hat{\bm{z}}_{.q}\hat{\bm{z}}_{.q}^T])  )]\\ &+E[\gamma_\epsilon]  \sum_{p:(p,q)\in \Psi_{\Omega}}  \mathcal{H}(\bm{Y}-\bm{E})_{p,q} [(E[\bm{s}_{.q}]\odot E[\hat{\bm{z}}_{.q}])^TE[\bm{d}_{p.}]^T]\\
&    +E[\text{ln}(\pi_k)]
\end{split}
\end{equation}
each entry in $\hat{z}_{.q}$ is the same with $z_{.q}$ except that $\hat{z}_{kq}=1$.

\begin{equation}
\begin{split}
&\text{ln}(\text{\bf{q}}(z_{kq}=0))\\
&\propto \frac{-E[\gamma_\epsilon]}{2} \sum_{p:(p,q)\in \Psi_{\Omega}}[\text{trace}(E[\bm{d}_{p.}^T\bm{d}_{p.}](E[\bm{s}_{.q} \bm{s}_{.q}^T ] \odot E[\hat{\bm{z}}_{.q}\hat{\bm{z}}_{.q}^T])  )] \\ &+E[\gamma_\epsilon]  \sum_{p:(p,q)\in \Psi_{\Omega}}     \quad \mathcal{H}(\bm{Y}-\bm{E})_{p,q} [(E[\bm{s}_{.q}]\odot E[\hat{\bm{z}}_{.q}])^TE[\bm{d}_{p.}]^T]\\
    &+E[\text{ln}(1-\pi_k)] \\
\end{split}
\end{equation}
each entry in $\hat{\bm{z}}_{.q}$ is the same with $\bm{z}_{.q}$ except that $\hat{z}_{kq}=0$.

And
\begin{equation} \label{updatepi1}
\begin{align}
&E[\text{ln}(\pi_k)]=\\
&\psi(\frac{a_0}{K}+\sum_{q=1}^{n_1}E[z_{kq}]) -\psi(\frac{a_0+b_0(K-1)}{K}+n_1)
\end{align}
\end{equation}

\begin{equation} \label{updatepi2}
\begin{align}
&E[\text{ln}(1-\pi_k)]=\\
&\psi(\frac{b_0(K-1)}{K}+n_1-\sum_{q=1}^{n_1}E[z_{kq}]) -\psi(\frac{a_0+b_0(K-1)}{K}+n_1)
\end{align}
\end{equation}

$\psi(.)$ is the diagamma  function.
 
\begin{equation}
    E[\bm{d}_{p.}^T\bm{d}_{p.}] = E[(\bm{d}_{p.})]^TE[(\bm{d}_{p.})]+\bm{\Sigma}_{\bm{d}_{p.}}\\
\end{equation}

\begin{equation}
     E[ \bm{s}_{.q}\bm{s}_{.q}^T] =  E[\bm{s}_{.q}]E[\bm{s}_{.q}]^T+\bm{\Sigma}_{\bm{s}_{.q}}
\end{equation}
\begin{equation}
     E[ \hat{\bm{z}}_{.q}\hat{\bm{z}}_{.q}^T] =  E[\hat{\bm{z}}_{.q}]E[\hat{\bm{z}}_{.q}]^T+\hat{\bm{\Sigma}}_{z_{.q}}
\end{equation}

And $\hat{\bm{\Sigma}}_{z_{.q}}=\text{diag}[E[z_{1q}](1-E[z_{1q}]),...,E[z_{Kq}](1-E[z_{Kq}])]$ $\hat{B}_kq=E[z_{kq}](1-E[z_{kq}])=0$

\noindent(IV) Sample $\pi_k$ ( $k=1,..., K$) from a Beta distribution

\begin{equation} \label{updatepi}
\begin{split}
&q(\pi_{k})  \sim \\ &\textrm{Beta}(\frac{a_0}{K}+\sum_{q=1}^{n_1}E[z_{kq}],\frac{b_0(K-1)}{K}+n_1-\sum_{q=1}^{n_1}E[z_{kq}])
 \end{split}
\end{equation}

\noindent(V) The probablistic density of $\gamma_s$  is a Gamma distribution
% $\gamma_s^c$ can be drawn from:

\begin{equation} \label{updategammas}
q(\gamma_s) \sim \Gamma(\frac{n_1K}{2}+c_0,\frac{1}{2}\sum_{q=1}^{n_1}E[s_{.q}^Ts_{.q}]+d_0) 
\end{equation}
with mean
\begin{equation} \label{updategammas2}
E[\gamma_s]=\frac{\frac{n_1K}{2}+c_0}{\frac{1}{2}\sum_{q=1}^{n_1}E[\bm{s}_{.q}^T\bm{s}_{.q}]+d_0)} 
\end{equation}
where
$E[\bm{s}_{.q}^T\bm{s}_{.q}] =  E[\bm{s}_{.q}^T] E[\bm{s}_{.q}]  +\text{trace}(\bm{\Sigma}_{\bm{s}_{.q}})$

\noindent(VI) The probablistic density of $E_{i,j}$  is a Gaussian distribution

\begin{equation}  \label{updateE}
q(E_{i,j}) \sim  \mathcal{N}(E[{E_{i,j}],\bm{\Sigma}_{E_{i,j}})
\end{equation}

\begin{equation}
\bm{\Sigma}_{E_{i,j}}=\frac{1}{E(\gamma_\epsilon)+E(\beta_{i,j})}
\end{equation}

\begin{equation} \label{updateE2}
E[{E_{i,j}]=E[\gamma_\epsilon]\Sigma_{E_{i,j}}(Y_{i,j}-E[(\mathcal{H}^{\dagger}\bm{X})_{ij}])
\end{equation}

where $E((\mathcal{H}^{\dagger}\bm{X})_{ij})=\frac{1}{\kappa_j}\sum_{(u, v) \in \Psi_{i, j}}[ E(d_{u.})(E(s_{.v}) \odot E(z_{.v}))]$

\noindent (VII)The approximation distribution over $\beta_{i,j}$ is a Gamma distribution

\begin{equation}\label{updatebeta}
 \beta_{i,j} \sim \Gamma(\frac{1}{2}+g_0,\frac{1}{2}E[E_{i,j}^2]+h_0) 
 \end{equation}
 
 with mean
 
 \begin{equation}\label{updatebeta2}
 E[\beta_{i,j}]=\frac{\frac{1}{2}+g_0}{\frac{1}{2}E[E_{i,j}^2]+h_0}
  \end{equation}

where $E[E_{i,j}^2] =  E[E_{i,j}] ^2 +\bm{\Sigma}_{E_{i,j}}$

\noindent(VI)The approximation distribution over $\gamma_{\epsilon}$ is a Gamma distribution
\begin{equation}\label{updateepsilon}
 q(\gamma_{\epsilon}|- ) \sim \Gamma( \frac{|\bm{\Omega}|}{2}+e_0,\frac{1}{2}E[||\bm{Y} -P_{\Omega} (\mathcal{H}^{\dagger}\bm{X}+\bm{E})||_F^2]+f_0).
 \end{equation}
 
 with mean
 \begin{equation}\label{updateepsilon2}
 E[\gamma_{\epsilon}]= \frac{ \frac{|\bm{\Omega}|}{2}+e_0}{ \frac{1}{2}E[||\bm{Y} -P_{\Omega} (\mathcal{H}^{\dagger}\bm{X}+\bm{E})||_F^2]+f_0}   
 \end{equation}

\subsection{Predictive mean and predictive variance}

 The predictive mean  can be computed as follows:

\begin{equation} 
\begin{split}\label{E1}
E[{\hat{\bm{x}}^c}]&=\int p({\hat{\bm{x}}^c}|\bm{\hat{x}},\bm{X},Y_{\Omega}){\hat{\bm{x}}^c}d{\hat{\bm{x}}^c}\\
                     &=\int (\int p({\hat{\bm{x}}^c}|\bm{\hat{x}},\bm{\Psi})p(\bm{\Psi}|\bm{X},\bm{Y}_\Omega)d\bm{\Psi}){\hat{\bm{x}}^c}d{\hat{\bm{x}}^c}\\
                     &=\int (\int p({\hat{\bm{x}}^c}|\bm{\hat{x}},\bm{\Psi}){\hat{\bm{x}}^c}d{\hat{\bm{x}}^c})p(\bm{\Psi}|\bm{X},\bm{Y}_\Omega)d\bm{\Psi}\\
                     &=\int E_{p({\hat{\bm{x}}^c}|\bm{\hat{x}},\bm{\Psi})}[{\hat{\bm{x}}^c}]p(\bm{\Psi}|\bm{X},\bm{Y}_\Omega)d\bm{\Psi}\\
                     &=\int f^{\bm{\Psi}}({\hat{\bm{x}}^c})p(\bm{\Psi}|\bm{X},\bm{Y}_\Omega)d\bm{\Psi}\\
                     &\approx\frac{1}{L}\sum_{l=1}^{l=L} f^{{{\bm{\Psi}}_l}}({\hat{\bm{x}}^c})  \quad {{\bm{\Psi}}_l} \sim p(\bm{\Psi}|\bm{X},\bm{Y}_\Omega)
\end{split}
\end{equation}
The predictive mean is the expectation for $\hat{x}^c$ over the probability $p({\hat{\bm{x}}^c}|\bm{\hat{x}},\bm{X},Y_{\Omega})$.} $\bm{\Psi}=\{\bm{D}^c, \hat{\bm{z}}^c, \hat{\bm{s}}^c, {\hat{y}^c},\hat{\gamma}_\epsilon\}$.   $f (\bm{\Psi})  = \bm{D}^c (\bm{\hat{z}^c} \odot \bm{\hat{s}^c})\hat{y}^c$. $E_{p({\hat{\bm{x}}^c}|\bm{\hat{x}},\bm{\Psi})}[{\hat{\bm{x}}^c}]$ denotes the expectation of $\hat{x}^c$ over the probability $p({\hat{\bm{x}}^c}|\bm{\hat{x}},\bm{\Psi})$.  The last step is because we sample ${\bm{\Psi}}_l}$  from $p(\bm{\Psi}|\bm{X},\bm{Y}_\Omega)$ and use Monte Carlo integration to compute it approximately.

In order to calculate the predictive covariance,  $E[{\hat{\bm{x}}^c}{\hat{\bm{x}}^c}^T]$ is derived as follows:
\begin{equation} 
\begin{split} \label{E2}
&E[{\hat{\bm{x}}^c}{\hat{\bm{x}}^c}^T]\\
&=\int p({\hat{\bm{x}}^c}|\bm{\hat{x}},\bm{X},Y_{\Omega}){\hat{\bm{x}}^c}{\hat{\bm{x}}^c}^Td{\hat{\bm{x}}^c}\\
&=\int (\int p({\hat{\bm{x}}^c}|\bm{\hat{x}},\bm{\Psi})p(\bm{\Psi}|\bm{X},\bm{Y}_\Omega)d\bm{\Psi}){\hat{\bm{x}}^c}{\hat{\bm{x}}^c}^T d{\hat{\bm{x}}^c}\\&=\int (\int p({\hat{\bm{x}}^c}|\bm{\hat{x}},\bm{\Psi}){\hat{\bm{x}}^c}{\hat{\bm{x}}^c}^Td{\hat{\bm{x}}^c})p(\bm{\Psi}|\bm{X},\bm{Y}_\Omega)d\bm{\Psi}\\&=\int (E_{p({\hat{\bm{x}}^c}|\bm{\hat{x}},\bm{\Psi})}[{\hat{\bm{x}}^c}{\hat{\bm{x}}^c}^T])p(\bm{\Psi}|\bm{X},\bm{Y}_\Omega)d\bm{\Psi}\\&=\int (\text{Var}_{p({\hat{\bm{x}}^c}|\bm{\hat{x}},\bm{\Psi})}[{\hat{\bm{x}}^c}]+E_{p({\hat{\bm{x}}^c}|\bm{\hat{x}},\bm{\Psi})}[{\hat{\bm{x}}^c}]{E_{p({\hat{\bm{x}}^c}|\bm{\hat{x}},\bm{\Psi})}[{\hat{\bm{x}}^c}]}^T ) \\
&\quad \quad \cdot p(\bm{\Psi}|\bm{X},\bm{Y}_\Omega)d\bm{\Psi}\\
&=\int (\frac{1}{C \hat{\gamma}_{\epsilon}}\bm{I}_P +{f^{\bm{\Psi}}({\hat{\bm{x}}^c})}{f^{\bm{\Psi}}({\hat{\bm{x}}^c})}^T)p(\bm{\Psi}|\bm{X},\bm{Y}_\Omega)d\bm{\Psi}  \\
& \approx  \frac{\bm{I}_P}{LC}\sum_{l=1}^{l=L} \frac{1}{\hat{\gamma}_{\epsilon}^{l}} +\frac{1}{L}\sum_{l=1}^{l=L} {f^{{{\bm{\Psi}}_l}}({\hat{\bm{x}}^c})}{f^{{{\bm{\Psi}}_l}}({\hat{\bm{x}}^c})}^T  \quad {{\bm{\Psi}}_l} \sim p(\bm{\Psi}|\bm{X},\bm{Y}_\Omega)
\end{split}
\end{equation}
 Plug (\ref{E1}) and (\ref{E2}) into equation (\ref{predictvariance}), we could obtain the predictive covariance in equation (\ref{predictvariance}).  
%where
%\begin{equation} \label{eq1}
%\begin{split}
%&E_{p({\hat{\bm{x}}^c}|\bm{\hat{x}},\bm{\Psi})}[{\hat{\bm{x}}^c}{\hat{\bm{x}}^c}^T]\\
%&=\text{Var}_{p({\hat{\bm{x}}^c}|\bm{\hat{x}},\bm{\Psi})}[{\hat{\bm{x}}^c}]+E_{p({\hat{\bm{x}}^c}|\bm{\hat{x}},\bm{\Psi})}[{\hat{\bm{x}}^c}]{E_{p({\hat{\bm{x}}^c}|\bm{\hat{x}},\bm{\Psi})}[{\hat{\bm{x}}^c}]}^T \\
%&= \frac{1}{C \hat{ \gamma}_{\epsilon}}\bm{I}_P +{f^{\bm{\Psi}}({\hat{\bm{x}}^c})} {f^{\bm{\Psi}}({\hat{\bm{x}}^c})}^T\\
%\end{split}
%\end{equation}
